# Supplementary material for: Unifying and extending Precision Recall metrics for assessing generative models
Source: arXiv:2405.01611 source file (2024-05-02)
Supplement: Supplementary file 1 [file 10_appendix.tex]

\section{Experiment with truncation trick performed on multi-variate Gaussians}

\juju{This is after ICML submission, following the rebuttal discussion}

Here we consider the synthetic case in $\R^d$ where
$$
P \sim \mathcal N (0, Id)
$$
and 
$$
Q_\psi \sim \mathcal N (0, \psi^2 Id)
$$
such that, the probability density functions write
$$
    dQ_\psi(x) = \frac{1}{(2\pi)^{d/2} \psi^d} \exp ( - \tfrac12 \Vert x \rVert^2/\psi^2 )  dx
$$
and
$$
d P(x) = d Q_1(x) = g(\|x\|)dx := \frac{1}{(2\pi)^{d/2}} \exp ( - \tfrac12 \Vert x \rVert^2 )  dx
$$

The likelihood-ratio $r_\psi = \frac{dP}{dQ}$ 
$$
    r_\psi(x)  
        = \psi^{d}  \exp (-\tfrac12 \Vert x \rVert^2 (1 - 1/\psi^2) ) 
        %= \Pi_{i=1}^d \, g_\psi(x_i)
        = g_\psi(\|x\|)^d
$$
is isotropic, with
$$
    y \ge 0 \mapsto h_\psi(y) 
    = \psi \exp (-\tfrac12 y^2 (1 - 1/\psi^2) ) 
    .
$$
\juju{à exprimer en fonction de P(x) ou $Q_\psi(x)$ ?}

Recall that precision and recall writes
\begin{equation*}
\begin{split}
    \alpha_{\lambda}(P,Q_\psi) 
    & =  \lambda \cdot \fpr(f_\lambda) + \fnr(f_\lambda) \\
    \beta_{\lambda}(P,Q_\psi) 
    &= \alpha_{\lambda} /  \lambda  
\end{split}
\end{equation*}
where 
\begin{align*}
    \fpr(f_\lambda) &= \int_{\R^d} (1-f_\lambda(x)) dP (x) 
    %\text{ and } 
    \\
    \fnr(f_\lambda) &=\int_{\R^d} f_\lambda(x) dQ_\psi(x)
\end{align*}
and where
$$
    f_\lambda (x)
        = \1_{r_\psi(x) \ge \frac{1}{\lambda}}
        = \1_{h_\psi(\|x\| )\ge \frac{1}{\lambda^{1/d}}}
$$
i.e. $f_\lambda(x) = 1 $ for data point $x$ s.t. $\lambda P(x) > Q_\psi(x)$, that is 
$$
   h_\psi(\|x\|)>\frac{1}{\lambda^{1/d}} 
   \Rightarrow 
   %\boxed{
   \|x\| \ge T_\psi(\lambda) = \sqrt{ \frac{2 \psi^2}{1-\psi^2} \log \frac \psi {\lambda^{1/d}} }
   %}
$$

Using $P=Q_1$ and appropriate change of variable ($z=x/\psi$ s.t. $d Q_\psi(x) = d P(x/\psi) = \frac1{(2\pi)^{d/2}} e^{-\tfrac 12 \|\frac x\psi\|^2} d(x/\psi))$, we get
\begin{align*}
    \fpr(f_\lambda) &= \int_{\R^d} (1-f_\lambda(x)) dP(x) 
    = 1 -  \int_{\R^d} f_\lambda(x) dP(x) 
    \\
    \fnr(f_\lambda) &=\int_{x \in \R^d} f_\lambda(x) dP(x/\psi)
        =\int_{z \in \R^d} f_\lambda(\psi x) dP(z)
\end{align*}

Using separability/isotropy, we have
$$
    \fnr(f_\lambda) 
        = \int_{x \in \R^d} f_\lambda( \psi x) dP(x)
        = \|\mathbb S^{d-1}\| \int_{\psi r \ge T_\psi(\lambda)} r^{d-1} g(r) dr 
$$
where the area of the hyper unit-sphere is
$$
S_{d-1} = \|\mathbb S^{d-1}\| =\frac {2\pi ^{d/2}}{\Gamma (\tfrac {d}{2} )}
$$.
The rightmost integral would be the $d-1$ moment of the centered 1D gaussian distribution if not for the lower bound $T_\psi(\lambda) / \psi$.

Similarly, we obtain
$$
    \fpr(f_\lambda)
        = 1 - \|\mathbb S^{d-1}\| \int_{r \ge T_\psi(\lambda)} r^{d-1} g(r) dr 
$$

In both case we have to compute the integral 
$$
    I_\psi(t) = I_{d-1} = \int_{r \ge t} r^{d-1} g(r) dr 
$$
and
$$
    \alpha(\lambda) = \lambda (1 - S_{d-1} I_\psi(T_\psi(\lambda))) 
    + S_{d-1} I_\psi(T_\psi(\lambda) / \psi)
$$

Using the fact that $g(r) = C e^{-r^2/2}$ and $g'(r) = -r g(r)$, 
integration by parts yields
\begin{align*}
    I_{d-1} 
    &= - \int_{r \ge t} r^{d-2} g'(r) dr 
    \\
    &= [ - 0 + t^{d-2} g(t) ] + (d-2) \int_{r \ge t} r^{d-3} g(r) dr 
    \\
    & = t^{d-2} g(t) + (d-2) I_{d-3}
\end{align*}
Recurrence shows that $ I_{d-1} $ is a polynomial expression of $t$ and is proportional to $g(t)$
$$
 I_{d-1} = g(t) P_d(t) 
$$

\juju{A finir ...}

\juju{Alternative par les bornes de Chernoff :
[1] Frank Nielsen. Generalized Bhattacharyya and Chernoff upper bounds on Bayes error using quasiarithmetic means. Pattern Recognition Letters, 42(0):25 – 34, 2014.}

$$
\alpha_\lambda = \int \min (\lambda P,Q) \le \int (\lambda P)^{\gamma} Q^{1-\gamma} = \mathbb E_Q \left( (\frac{\lambda P}{Q})^{\gamma} \right)
= \lambda^\gamma \mathbb E_Q \left( (\frac{ P}{Q})^{\gamma} \right)
$$
Avec des gaussiennes isotropes en dimension $d$ : $P = Q_1 = p{}^{\otimes d} $ et $Q_\psi = q {}^{\otimes d} = \mathcal N (0, \psi^2 I_d) = \mathcal N (0, \psi^2) {}^{\otimes d}$
on a la borne
$$
\alpha_\lambda \le \lambda^\gamma C(P,Q)^d = \lambda^\gamma {C(\mathcal N (0, 1),\mathcal N (0, \psi^2))}^d = = \lambda^\gamma C(p,q)^d
$$
où $C$ est le coefficient de Chernoff :
$$
C (P,Q) = inf_\gamma \mathbb E_Q (\frac{P}{Q})^{\gamma} 
$$
qui vaut 1 si $P=Q$ et 0 si $P \perp Q$

La divergence de Chernoff est $D_C = -\log C$ et est entre 0 et l'infini

le membre de droite de l'inégalité est une constante à la puissance d, soit
$$
\alpha_\lambda({p}^{\otimes d},{q}^{\otimes d}) \le \lambda^\gamma e^{-d D_C(p,q)}
$$

%C_\alpha()
